# Supplementary material for: CTD: Fast, Accurate, and Interpretable Method for Static and Dynamic Tensor Decompositions
Source: arXiv:1710.03608 source file (2017-10-09)
Supplement: Supplementary file 1 [file appendix.tex]

\begin{figure*} [t]
	\subfloat
	{	\includegraphics[width=0.32 \textwidth]{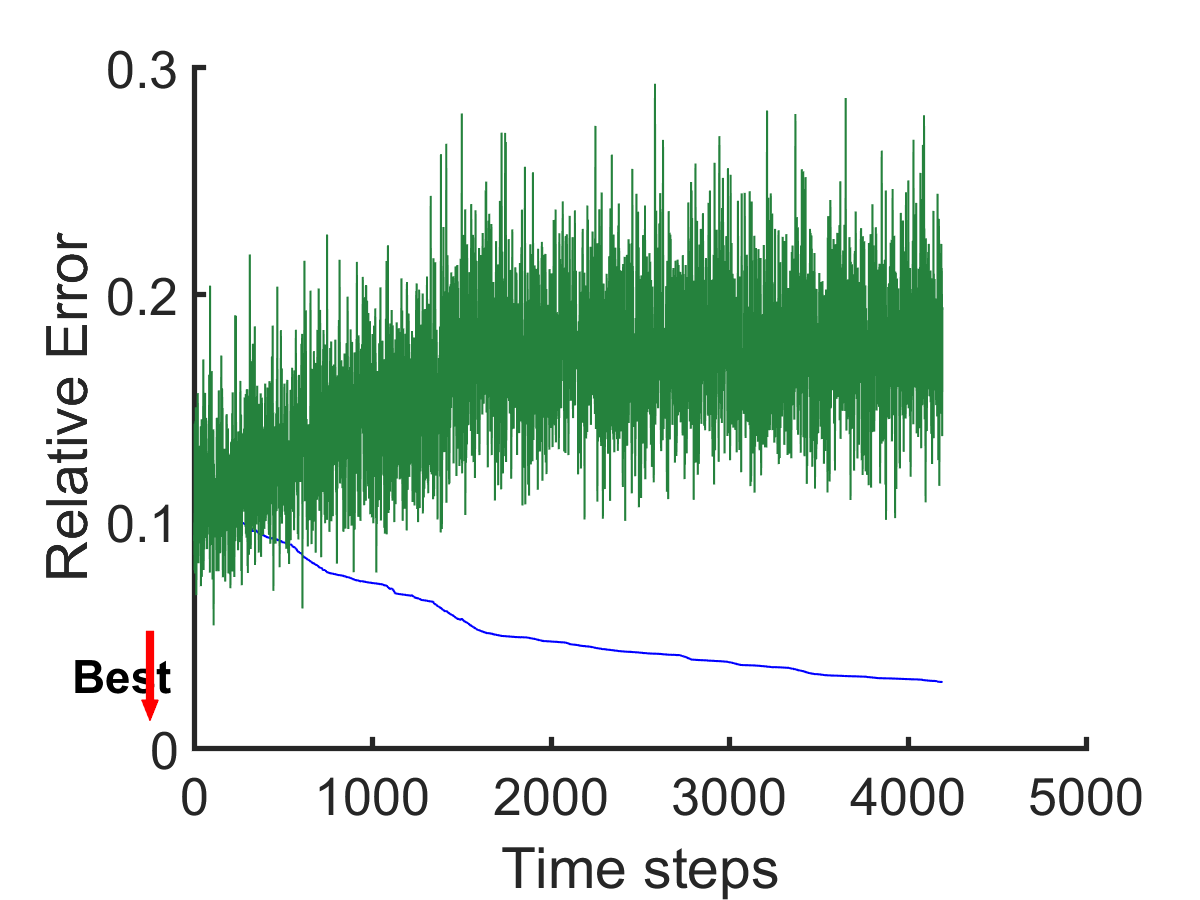}
	}
	\subfloat
	{	\includegraphics[width=0.32 \textwidth]{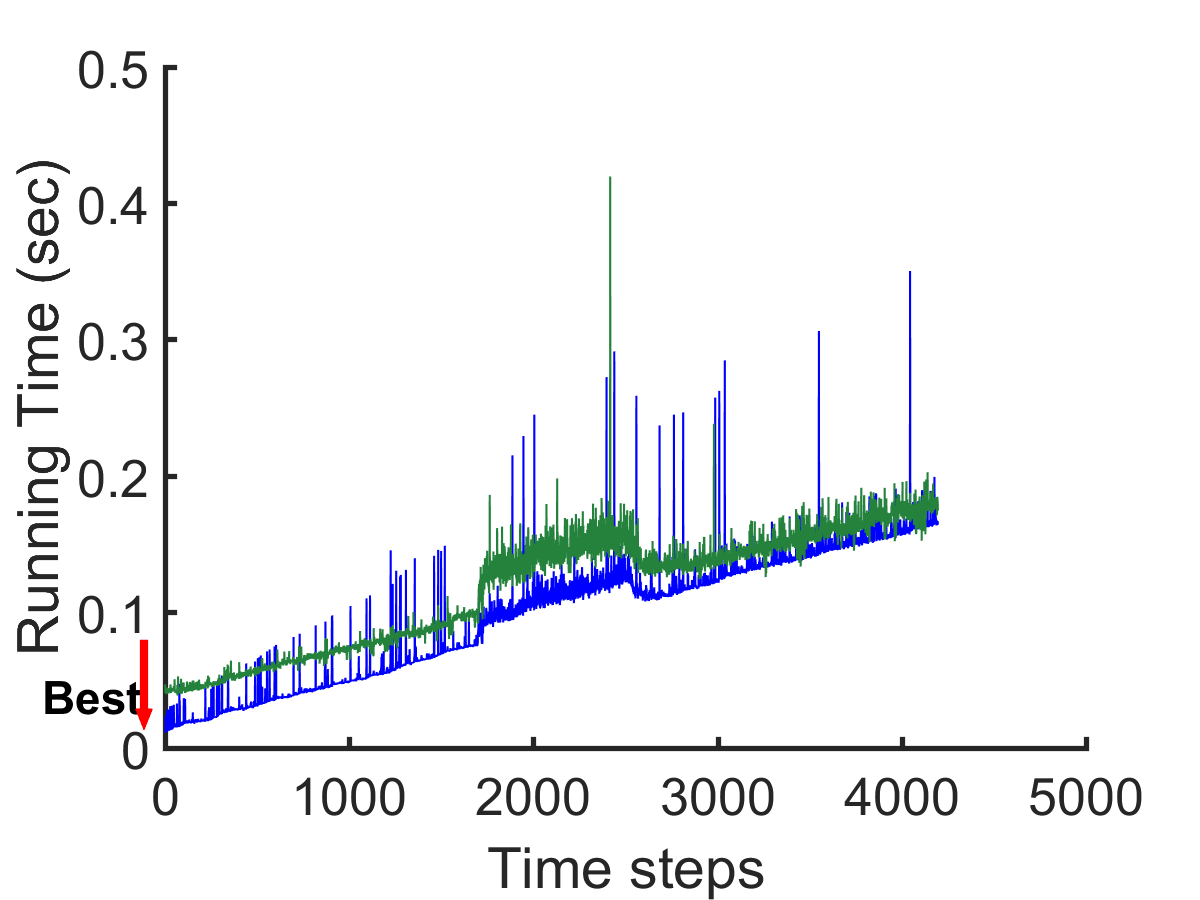}
	}
	\subfloat
	{	\includegraphics[width=0.32 \textwidth]{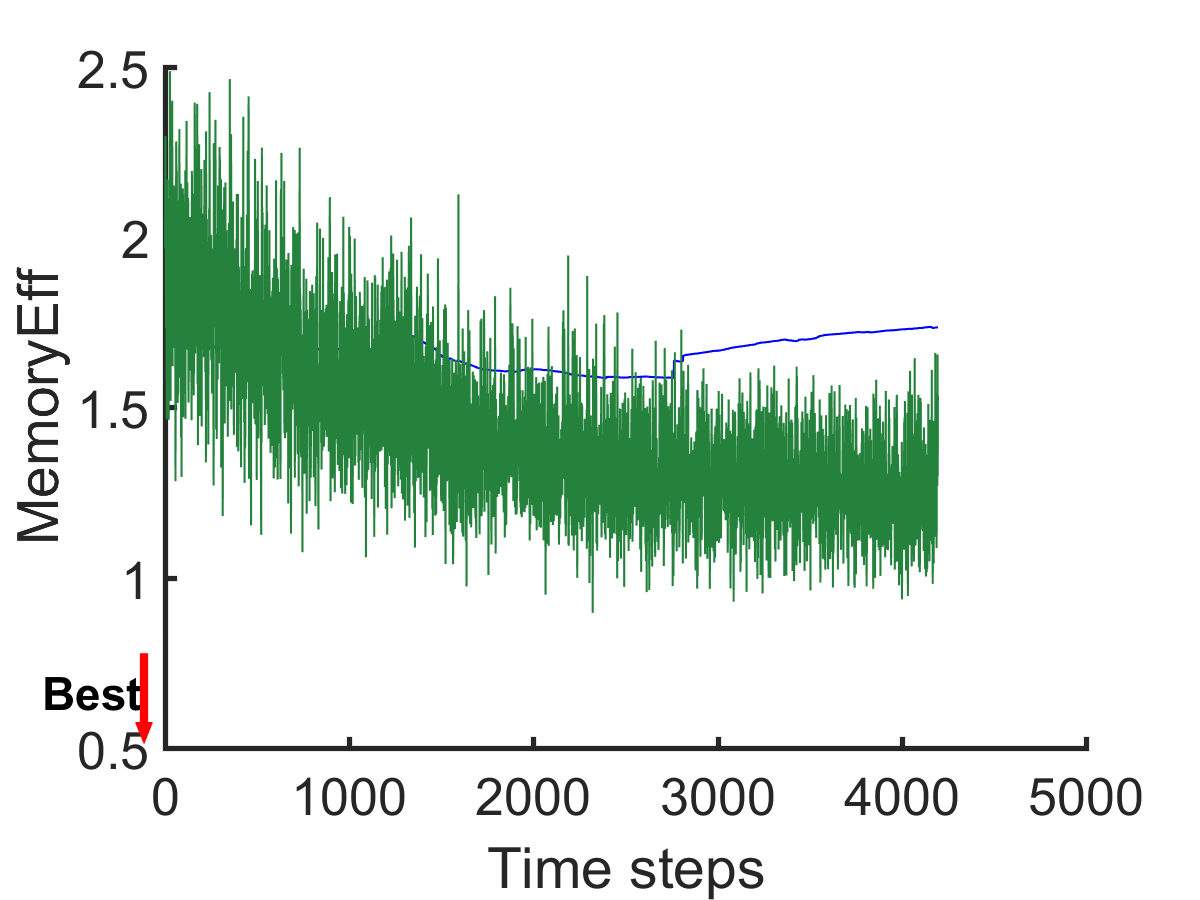}
	}
	\caption{Hypertext 2009}
\end{figure*}

\begin{figure*} [t]
	\subfloat
	{	\includegraphics[width=0.32 \textwidth]{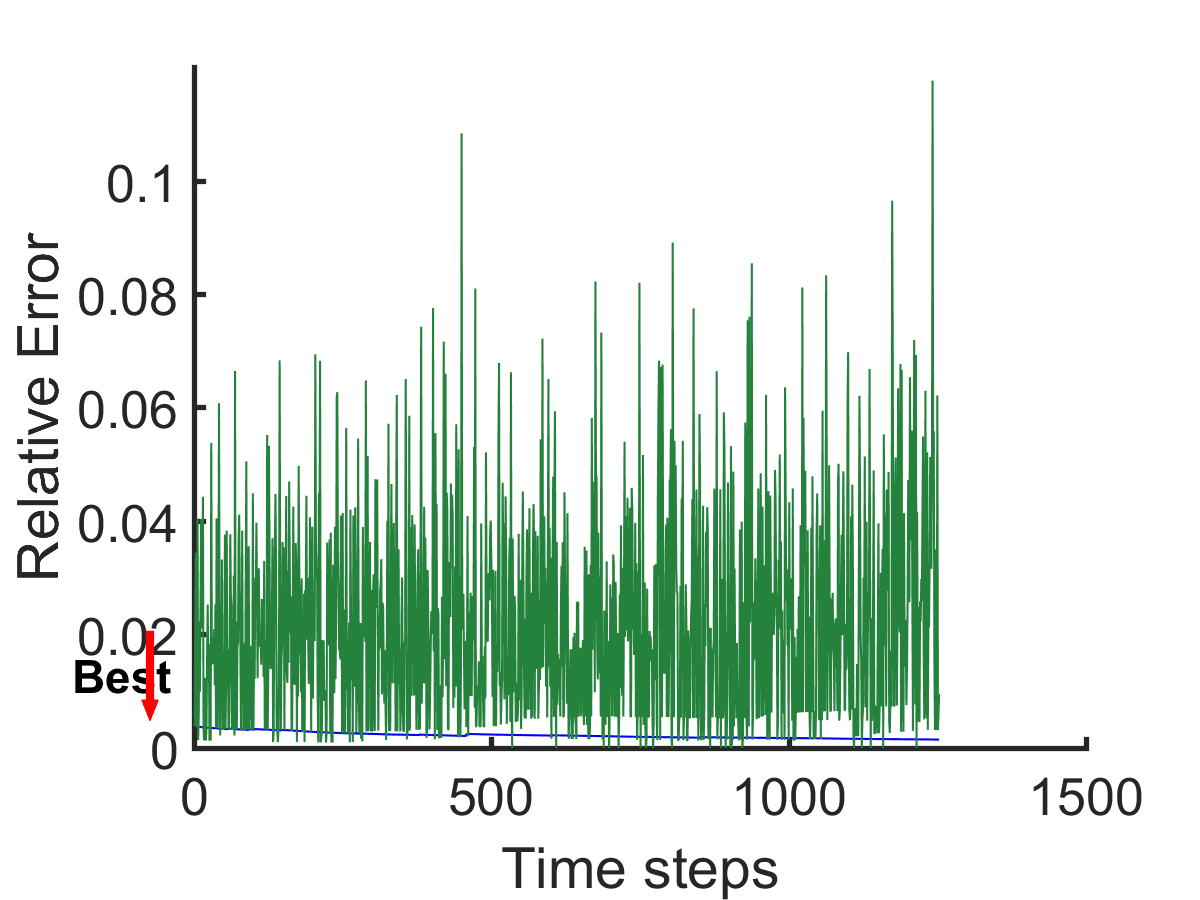}
	}
	\subfloat
	{	\includegraphics[width=0.32 \textwidth]{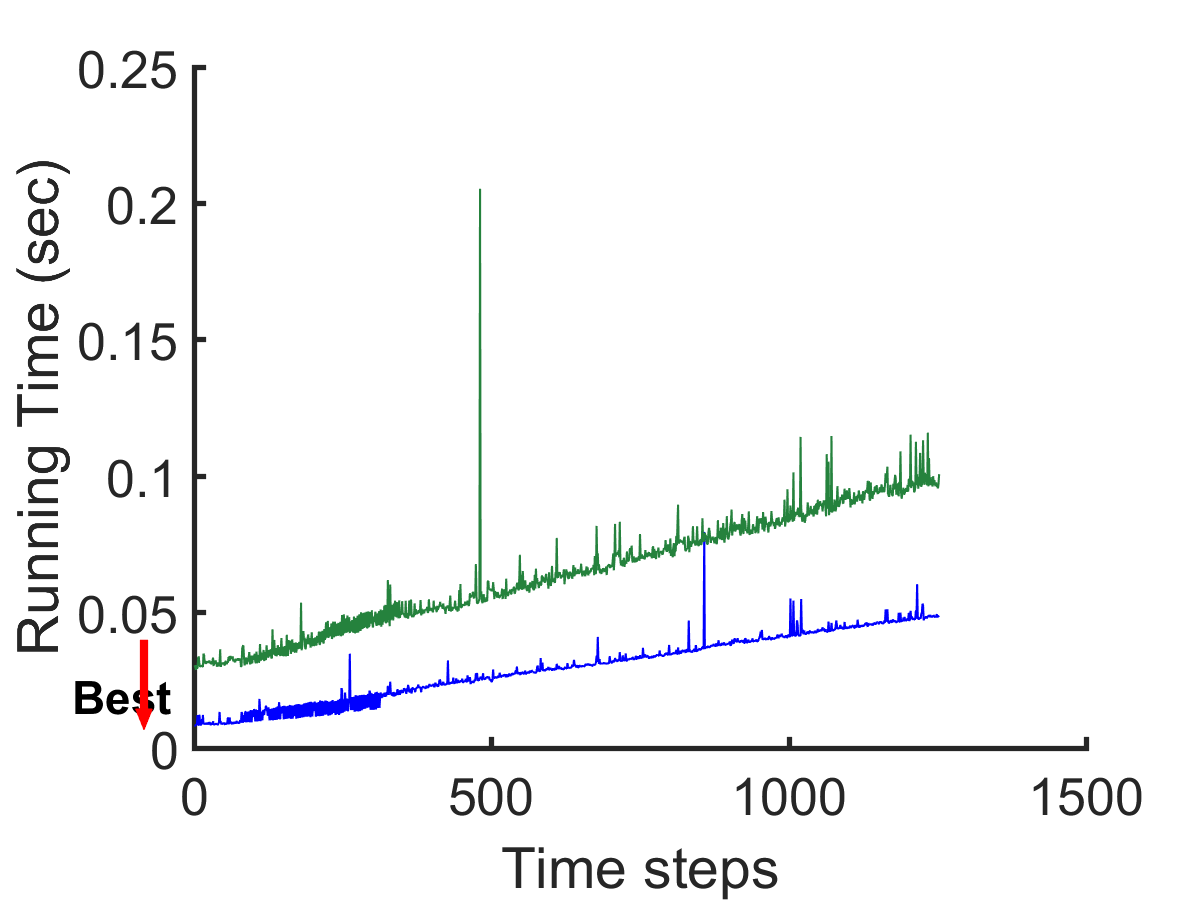}
	}
	\subfloat
	{	\includegraphics[width=0.32 \textwidth]{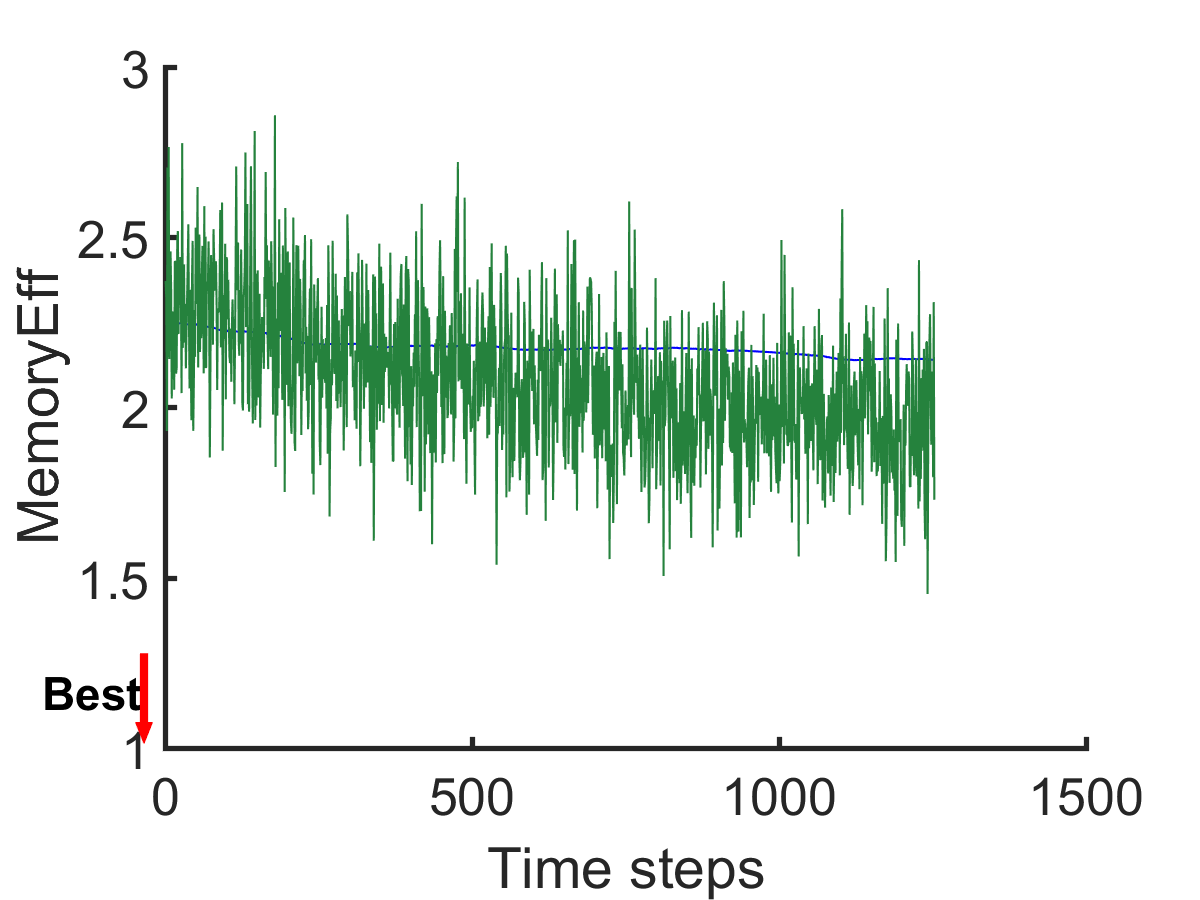}
	}
	\caption{Haggle}
\end{figure*}

\begin{figure*} [t]
	\subfloat
	{	\includegraphics[width=0.32 \textwidth]{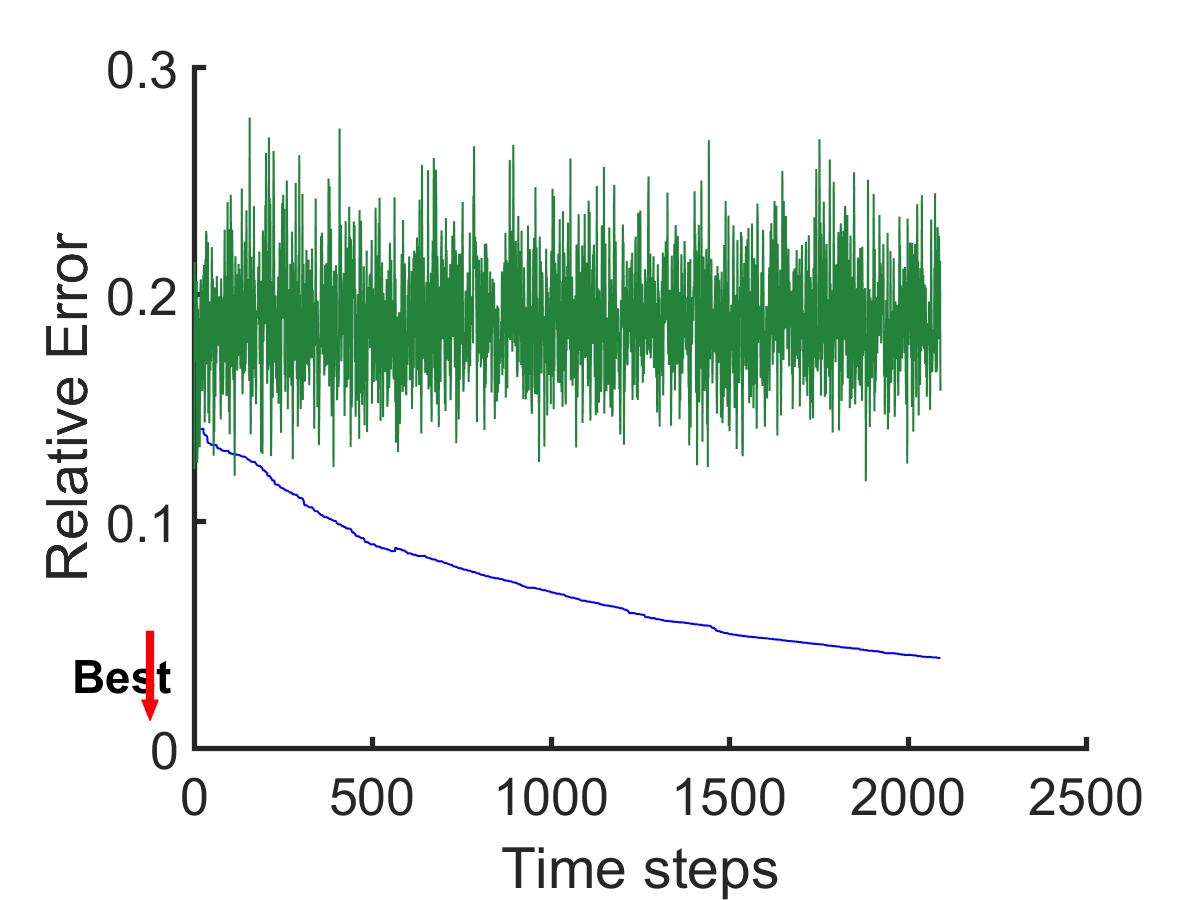}
	}
	\subfloat
	{	\includegraphics[width=0.32 \textwidth]{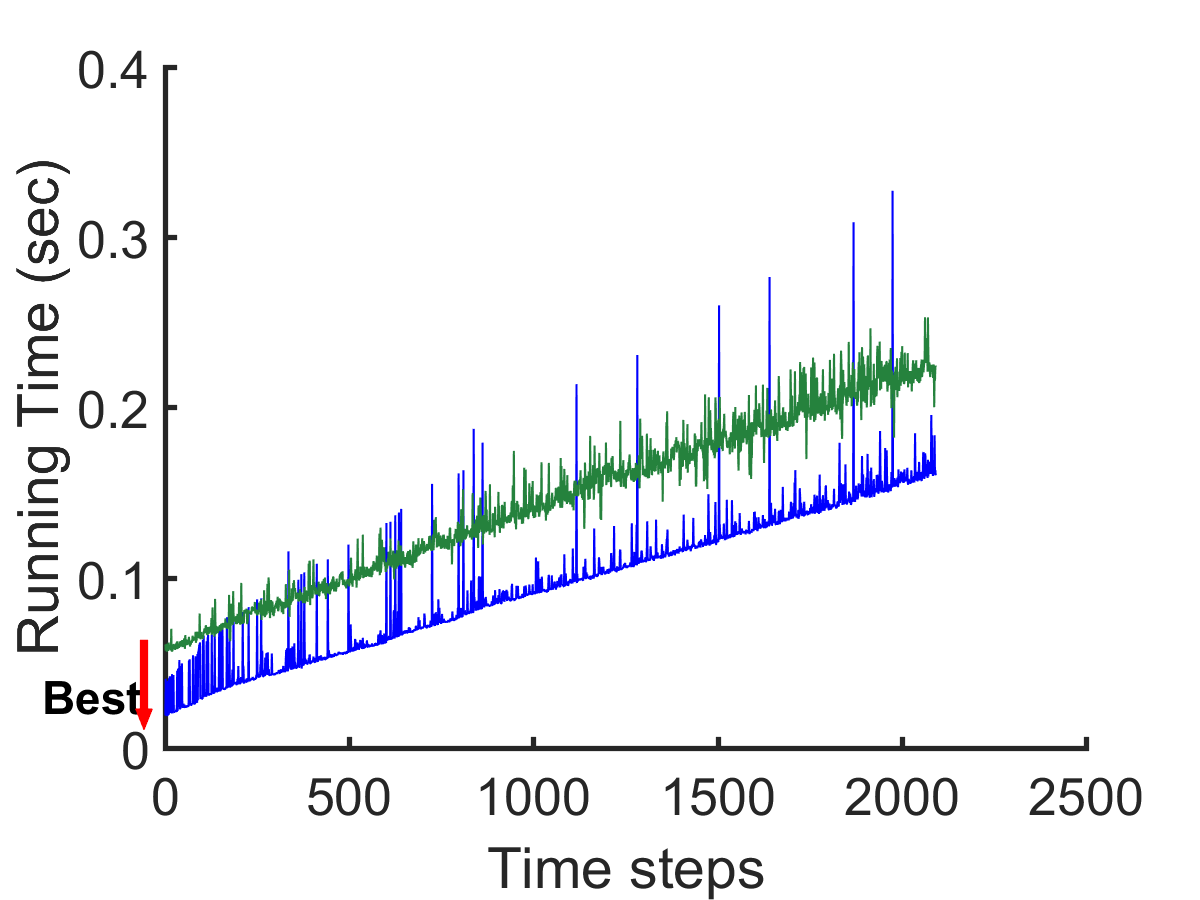}
	}
	\subfloat
	{	\includegraphics[width=0.32 \textwidth]{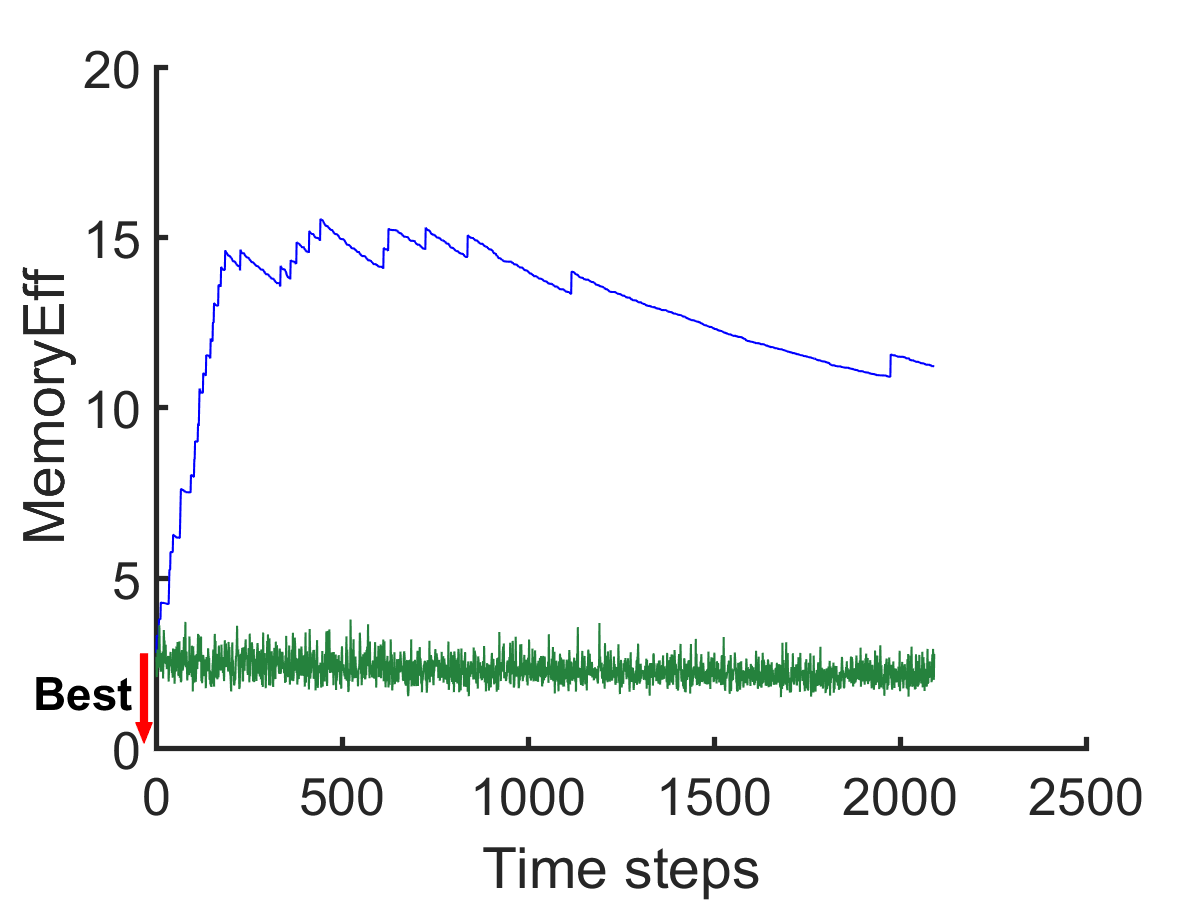}
	}
	\caption{Manufacturing Emails}
\end{figure*}

\begin{figure*} [t]
	\subfloat
	{	\includegraphics[width=0.32 \textwidth]{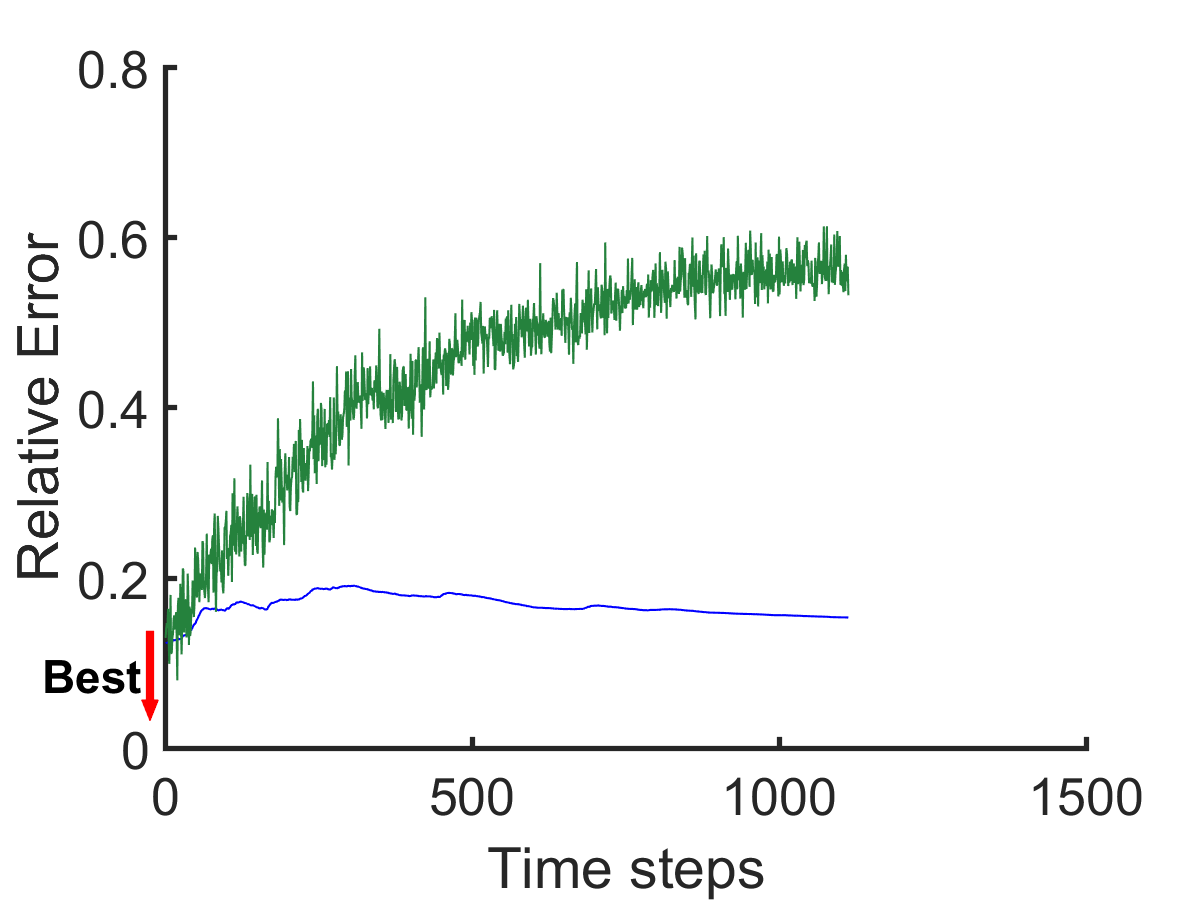}
	}
	\subfloat
	{	\includegraphics[width=0.32 \textwidth]{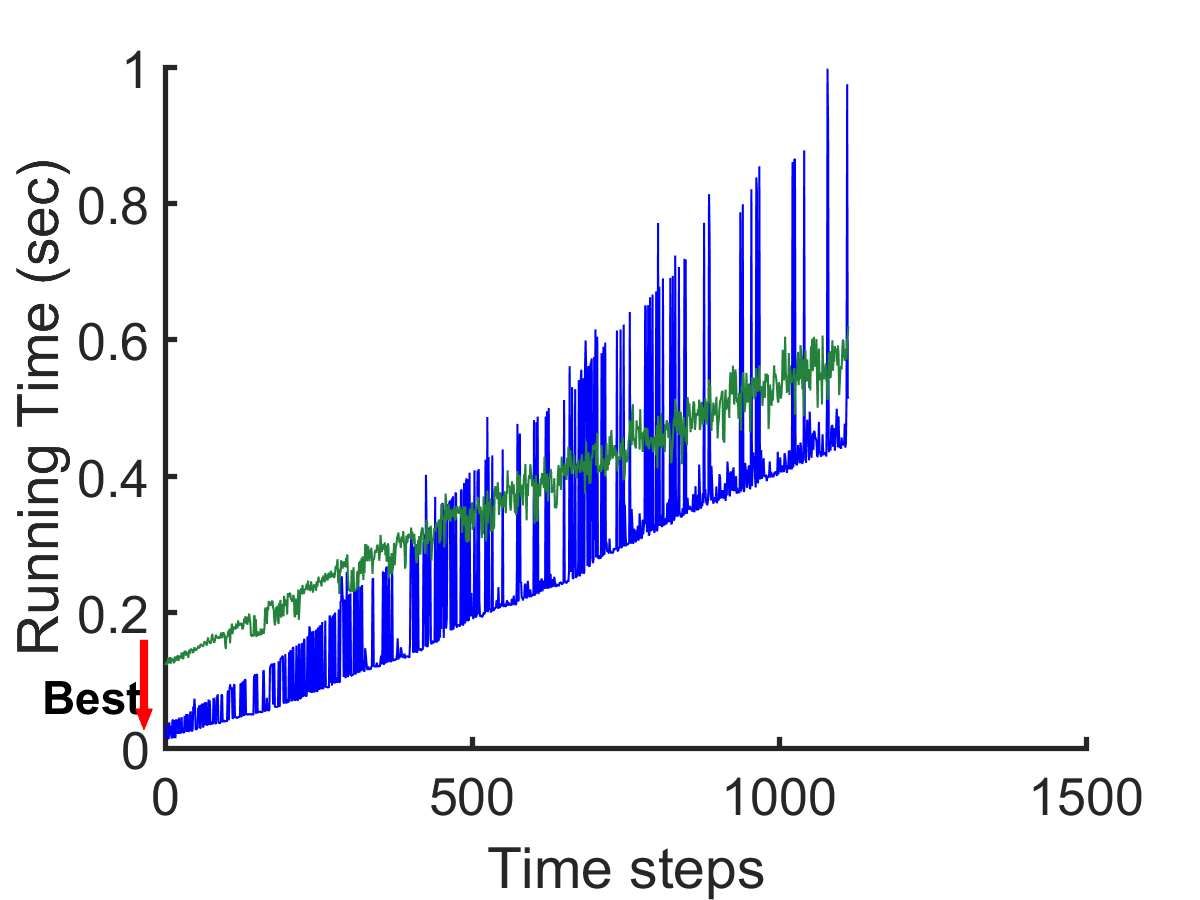}
	}
	\subfloat
	{	\includegraphics[width=0.32 \textwidth]{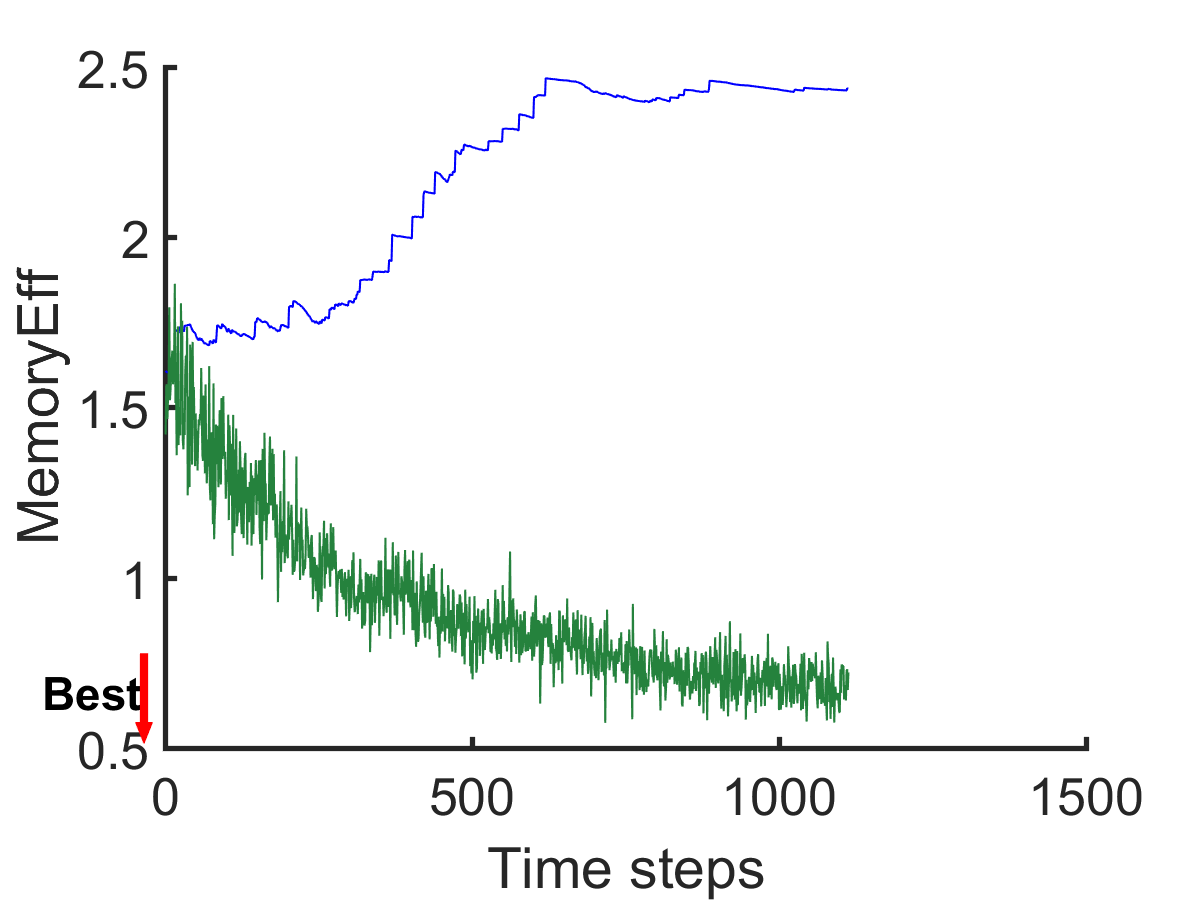}
	}
	\caption{Infectious}
\end{figure*}
